# Supplementary material for: Effect of modeling subject-specific cortical folds on brain injury risk prediction under blunt impact loading
Source: arXiv:2510.08379 source file (2025-11-06)
Supplement: Supplementary file 1 [file Supplementary_Materials_Effect_of_cortical_folds.pdf]

# Supplementary Materials: Effect of modeling subject-specific cortical folds on brain injury risk prediction under blunt impact loading

## S1 List of Acronyms

|              |                                                     |
|--------------|-----------------------------------------------------|
| <b>CORA</b>  | Correlation and Analysis                            |
| <b>CSDM</b>  | Cumulative Strain Damage Measure                    |
| <b>CSF</b>   | Cerebral Spinal Fluid                               |
| <b>DTI</b>   | Diffusion Tensor Imaging                            |
| <b>FE</b>    | Finite Element                                      |
| <b>MRI</b>   | Magnetic Resonance Imaging                          |
| <b>MPS</b>   | Maximum Principal Strain                            |
| <b>MPSR</b>  | Maximum Principal Strain Rate                       |
| <b>NDT</b>   | Neutral Density Target                              |
| <b>NHTSA</b> | U.S. National Highway Traffic Safety Administration |
| <b>PLA</b>   | Peak Linear Acceleration                            |
| <b>TBI</b>   | Traumatic Brain Injury                              |

## S2 Validation of the finite element head model

The FE head model was evaluated for deformation and strain prediction in brain tissue using experimental datasets: (a) cadaveric head impact tests by Hardy et al. [1], and (b) *in vivo* strain measurements from tagged MRI of mild head accelerations [2].

### S2.1 Validation against Hardy cadaveric head impact study

In this study, four tests from two subjects (Table S1) were selected from the cadaveric head impact tests of Hardy et al. [1] to evaluate the brain deformation response of the FE head model. In these tests, cadaveric heads were impacted at either the occipital region, the left-side temporal region, or the left-side parietal region. The skull-brain relative motion was captured by high-speed X-ray with two implanted clusters of neutral density targets (NDTs). The average tissue strains and NDT displacements from the experiments were reanalyzed by Zhou et al. [3, 4], and we used this reanalyzed data to evaluate our simulations (instead of the original data from Hardy et al.). In our simulations, the finite element model was scaled uniformly in each direction to match the head size of the experimental subjects, and the

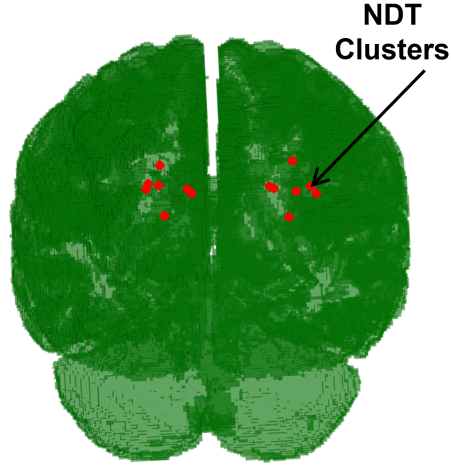

Figure S1: Representative NDT clusters location assignments of specimen C288 in the finite element model based on reported coordinates from Hardy et al. 2007 [1].

location of the NDTs was defined based on the reported initial locations [3] shown in Figure S1. The NDTs in each cluster were adjusted slightly such that all the NDTs were located in the brain tissue and the relative distance between the NDTs remained unchanged.

Table S1: Selected cadaveric experimental tests and subject dimensions from Hardy et al. 2007 [1] used to evaluate the FE model.

| Specimen and Test |    | Impact  | Plane      | Region       | Helmet | Head dimensions |         |
|-------------------|----|---------|------------|--------------|--------|-----------------|---------|
|                   |    |         |            |              |        | Depth           | Breadth |
| C288              | T3 | offset  | median     | occipital    | n      | 18.4 cm         | 13.3 cm |
| C380              | T2 | offset  | horizontal | parietal lt. | y      | 18.5 cm         | 16.0 cm |
|                   | T4 | offset  |            |              | n      |                 |         |
|                   | T6 | aligned | coronal    | temporal lt. | n      |                 |         |

The time history of average maximum principal strain (Green-Lagrange) at the NDT clusters and the NDT displacements were exported from the simulations and compared with the experimental data. CORA (Correlation and Analysis) scores that quantitatively compare the time history from the simulation results and the experimental data were evaluated using standard CORA parameters [5]. The results were plotted against results from other finite element models [3, 6, 7] as shown in Figures S2 - S6. The strain response of our FE model showed good agreement and high correlations with the experimental data, with CORA scores ranging from 0.693 (fair) to 0.910 (excellent), as shown in Figure S2. The CORA scores of the NDT displacements ranged from 0.40 (marginal) to 0.860 (excellent). The average CORA score of the NDT displacement falls within the fair and good categories of the biofidelity scale, as shown in Table S2.

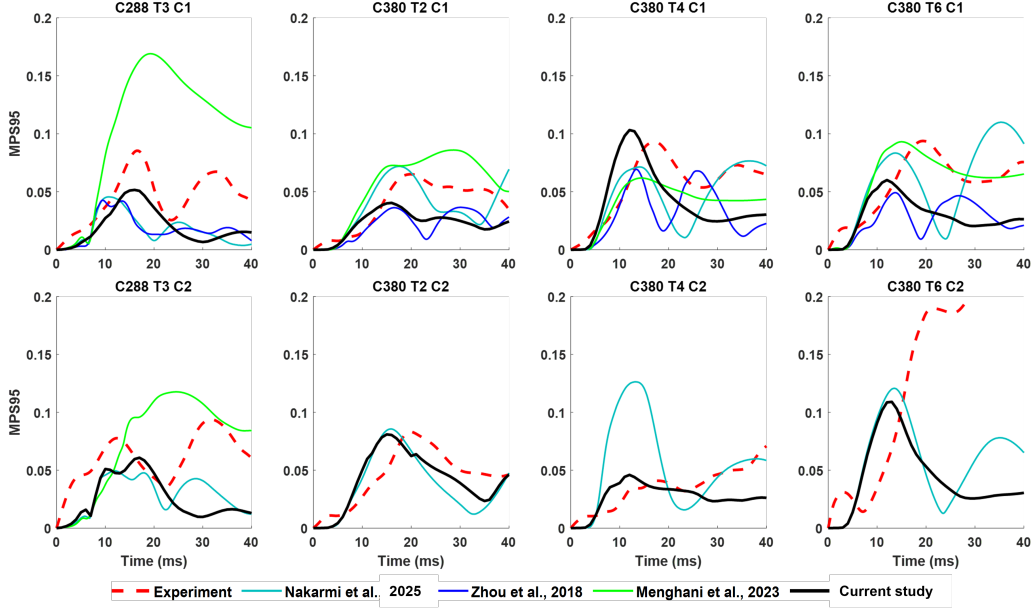

Figure S2: Comparison of the maximum principal strain of the NDT clusters between our simulated results and experimental results from Hardy et al. [3] and other finite element modeling studies [6, 3].

## S2.2 Validation against in vivo experiments using tagged MRI

The strain response of the finite element model was also compared to strains measured in an in vivo experiment of a mild, non-injurious head impact during neck rotation [2]. The angular velocity of the head and the direction of neck rotation simulated are shown in Figure S7. A qualitative comparison between the MPS contours of the tagged MRI experiment and simulation is shown in Figure S9a, along with a comparison to another FE head model validated under the same testing [7]. The quantitative comparison between the maximum principal strain (MPS) from the experiment and our simulation is shown in Figure S9b. The CORA score between the simulations and experimental MPS95 is found to be 0.674, which lies in the ‘fair’ range. At the very low strain and strain rates used in the experiment, the simulation under-predicts the principal strains. The peak MPS95 for the experiment and simulation are 0.038 and 0.019, respectively, highlighting the significantly stiffer response of the FE model compared to the in-vivo experiments, under such low strain loading. However, peaks MPS95 occurs at the same time instance (45 ms) both in the simulation and the experiment.

Table S2: CORA scores of NDT displacements compared with experimental results.

|                |       | C288T3  | C380T2  | C380T4  | C380T6  |
|----------------|-------|---------|---------|---------|---------|
| X-displacement | NDT1  | 0.747   | 0.487   | 0.771   | 0.669   |
|                | NDT2  | 0.77555 | 0.4835  | 0.77173 | 0.67966 |
|                | NDT3  | 0.74517 | 0.59206 | 0.77055 | 0.74118 |
|                | NDT4  | 0.58057 | 0.55822 | 0.83981 | 0.66229 |
|                | NDT5  | 0.61107 | 0.55145 | 0.84328 | 0.68553 |
|                | NDT6  | 0.61621 | 0.50858 | 0.83083 | 0.77571 |
|                | NDT7  | 0.50787 | 0.47078 | 0.63699 | 0.5962  |
|                | NDT8  | 0.49786 | 0.51413 | 0.8595  | 0.76486 |
|                | NDT9  | 0.83306 | 0.61351 | 0.65787 | 0.61511 |
|                | NDT10 | 0.61881 | 0.39951 | 0.57162 | 0.40227 |
|                | NDT11 | 0.84587 | 0.6843  | 0.6832  | 0.69564 |
|                | NDT12 | 0.58257 | 0.68988 | 0.73912 | 0.7488  |
|                | NDT13 | 0.52516 | 0.74059 | 0.77762 | 0.65912 |
|                | NDT14 | 0.79135 | 0.67091 | 0.68902 | 0.76004 |
| Y-displacement | NDT1  | 0.456   | 0.59    | 0.423   | 0.377   |
|                | NDT2  | 0.77555 | 0.4835  | 0.77173 | 0.67966 |
|                | NDT3  | 0.74517 | 0.59206 | 0.77055 | 0.74118 |
|                | NDT4  | 0.58057 | 0.55822 | 0.83981 | 0.66229 |
|                | NDT5  | 0.61107 | 0.55145 | 0.84328 | 0.68553 |
|                | NDT6  | 0.61621 | 0.50858 | 0.83083 | 0.77571 |
|                | NDT7  | 0.50787 | 0.47078 | 0.63699 | 0.5962  |
|                | NDT8  | 0.49786 | 0.51413 | 0.8595  | 0.76486 |
|                | NDT9  | 0.83306 | 0.61351 | 0.65787 | 0.61511 |
|                | NDT10 | 0.61881 | 0.39951 | 0.57162 | 0.40227 |
|                | NDT11 | 0.84587 | 0.6843  | 0.6832  | 0.69564 |
|                | NDT12 | 0.58257 | 0.68988 | 0.73912 | 0.7488  |
|                | NDT13 | 0.52516 | 0.74059 | 0.77762 | 0.65912 |
|                | NDT14 | 0.79135 | 0.67091 | 0.68902 | 0.76004 |
| Z-displacement | NDT1  | 0.638   | 0.637   | 0.551   | 0.652   |
|                | NDT2  | 0.77555 | 0.4835  | 0.77173 | 0.67966 |
|                | NDT3  | 0.74517 | 0.59206 | 0.77055 | 0.74118 |
|                | NDT4  | 0.58057 | 0.55822 | 0.83981 | 0.66229 |
|                | NDT5  | 0.61107 | 0.55145 | 0.84328 | 0.68553 |
|                | NDT6  | 0.61621 | 0.50858 | 0.83083 | 0.77571 |
|                | NDT7  | 0.50787 | 0.47078 | 0.63699 | 0.5962  |
|                | NDT8  | 0.49786 | 0.51413 | 0.8595  | 0.76486 |
|                | NDT9  | 0.83306 | 0.61351 | 0.65787 | 0.61511 |
|                | NDT10 | 0.61881 | 0.39951 | 0.57162 | 0.40227 |
|                | NDT11 | 0.84587 | 0.6843  | 0.6832  | 0.69564 |
|                | NDT12 | 0.58257 | 0.68988 | 0.73912 | 0.7488  |
|                | NDT13 | 0.52516 | 0.74059 | 0.77762 | 0.65912 |
|                | NDT14 | 0.79135 | 0.67091 | 0.68902 | 0.76004 |
| Average        |       | 0.6562  | 0.5752  | 0.7439  | 0.6759  |

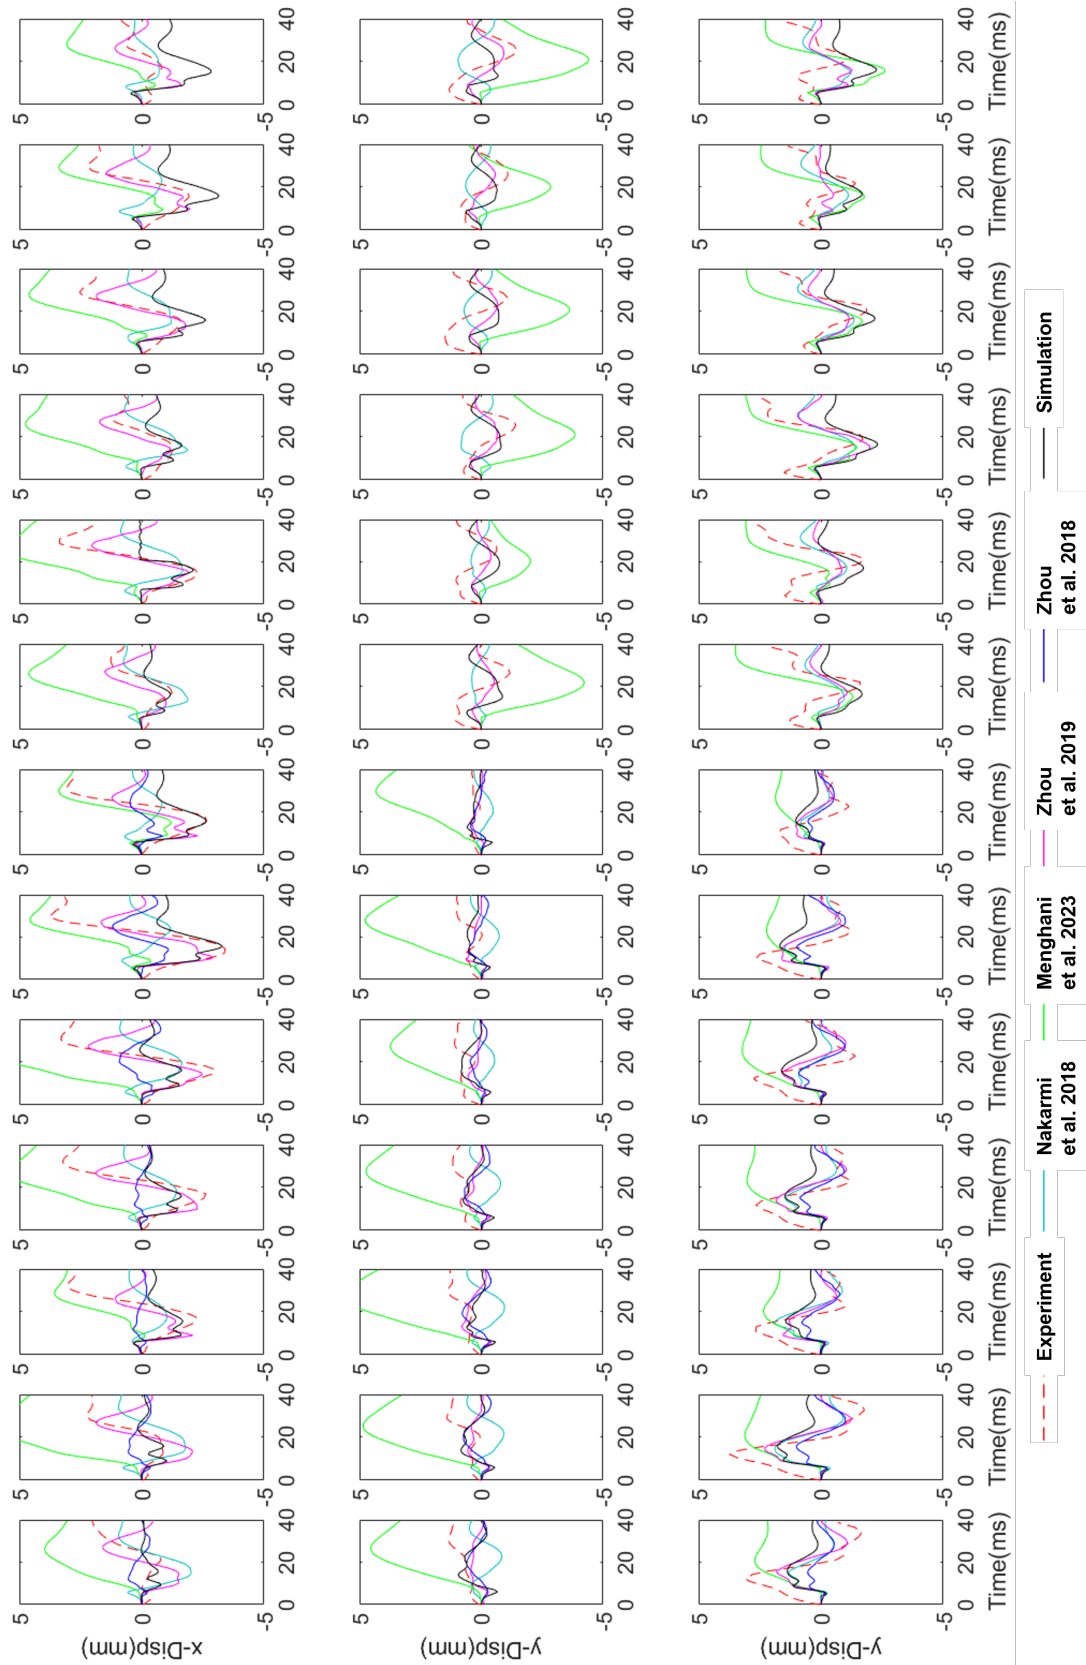

Figure S3: Comparison of NDT displacements between our simulated results and experimental results from Hardy [4] and other FEA studies [4, 6, 3, 7] for test case C288-T3.

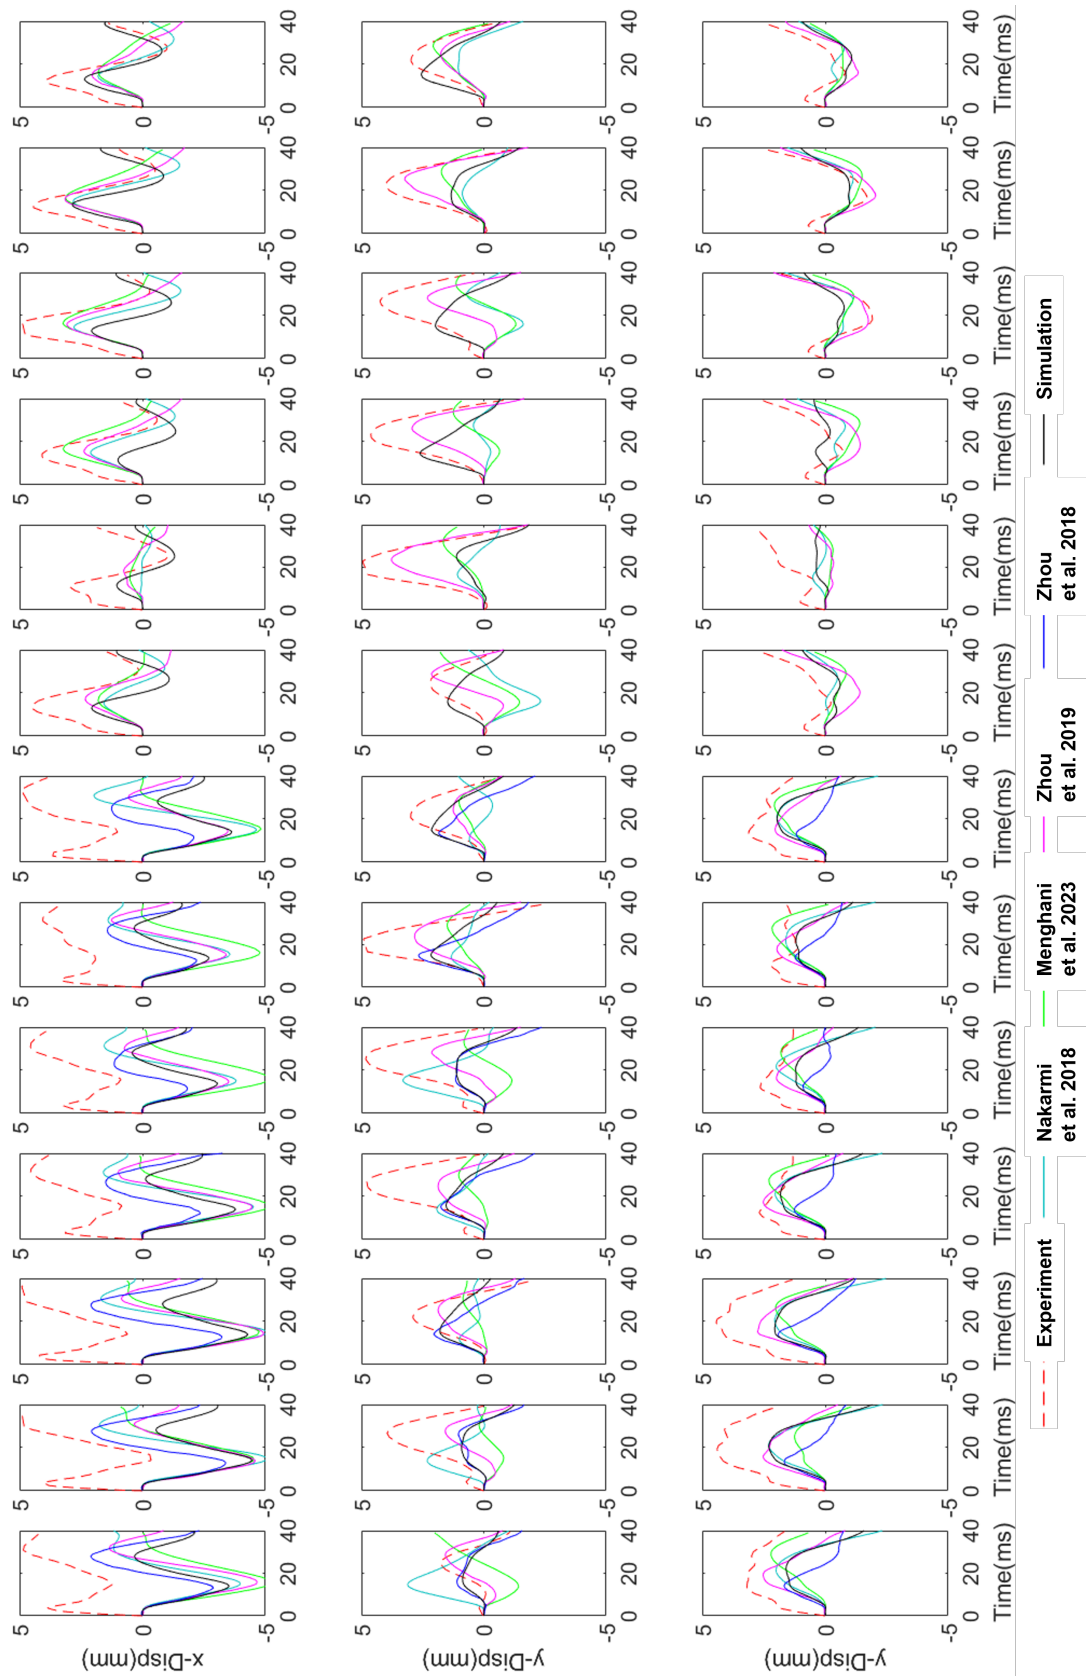

Figure S4: Comparison of NDT displacements between our simulated results and experimental results from Hardy [4] and other FEA studies [4, 6, 3, 7] for test case C380-T2.

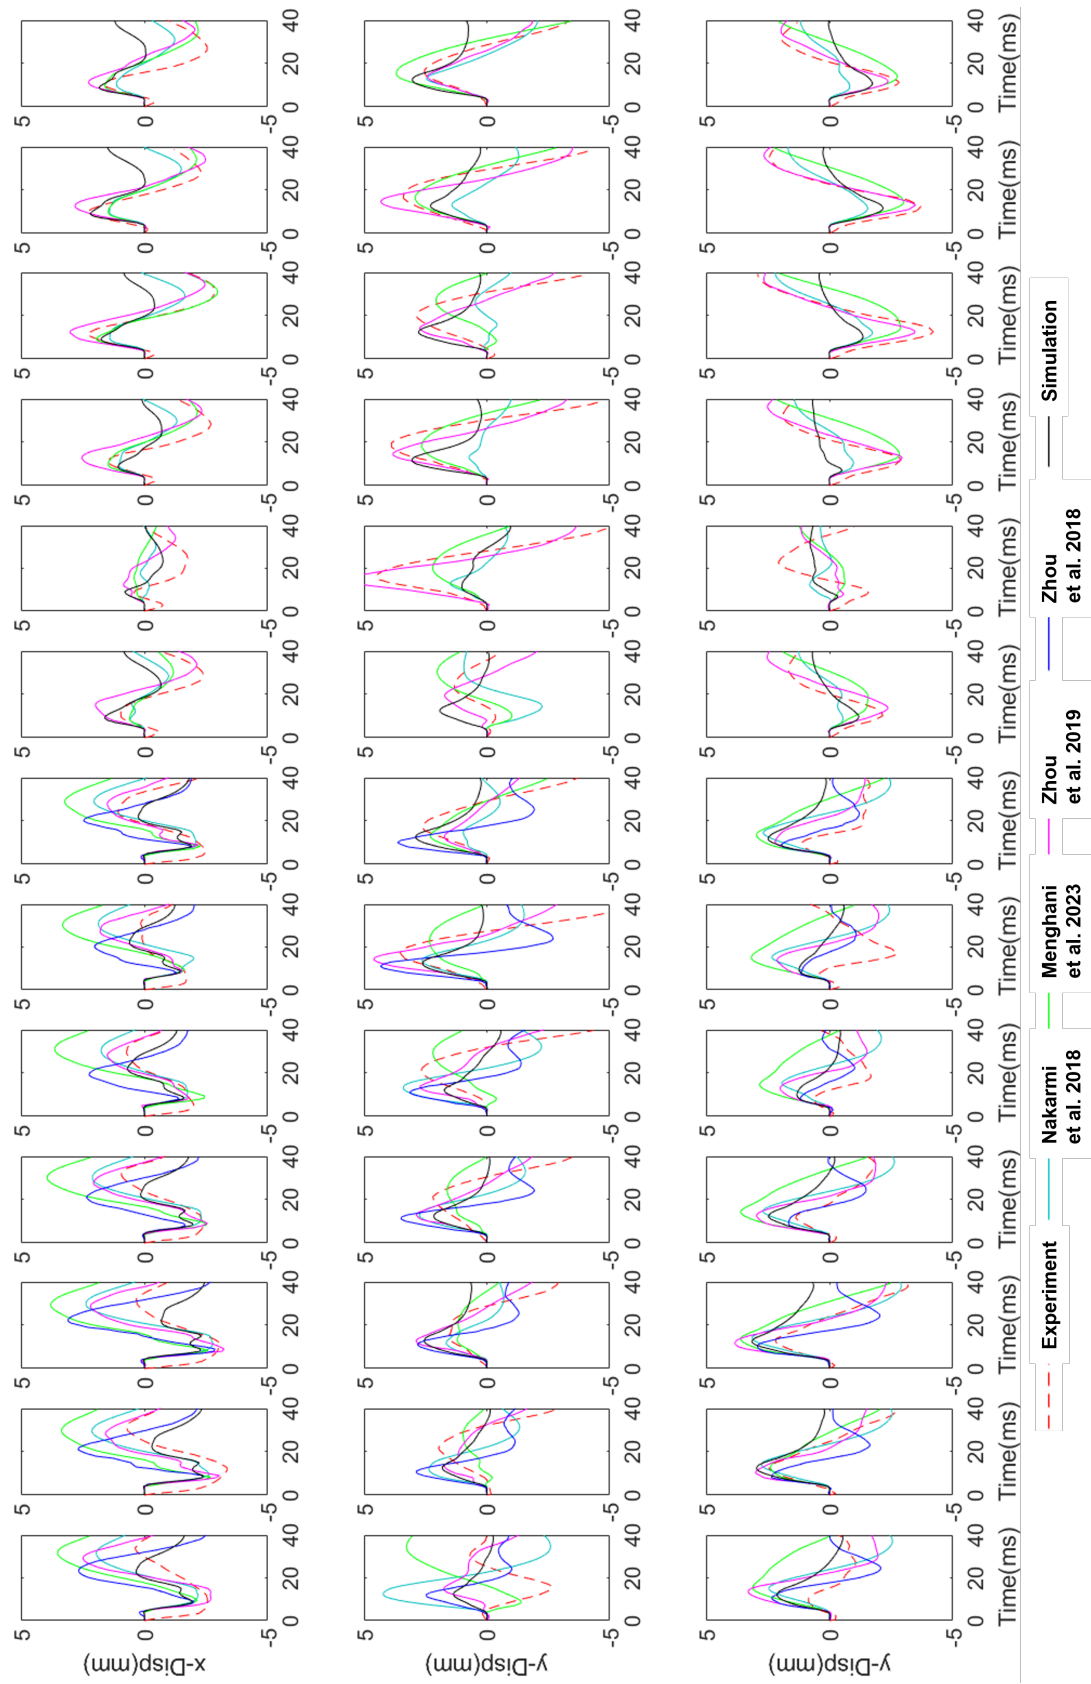

Figure S5: Comparison of NDT displacements between our simulated results and experimental results from Hardy [4] and other FEA studies [4, 6, 3, 7] for test case C380-T4.

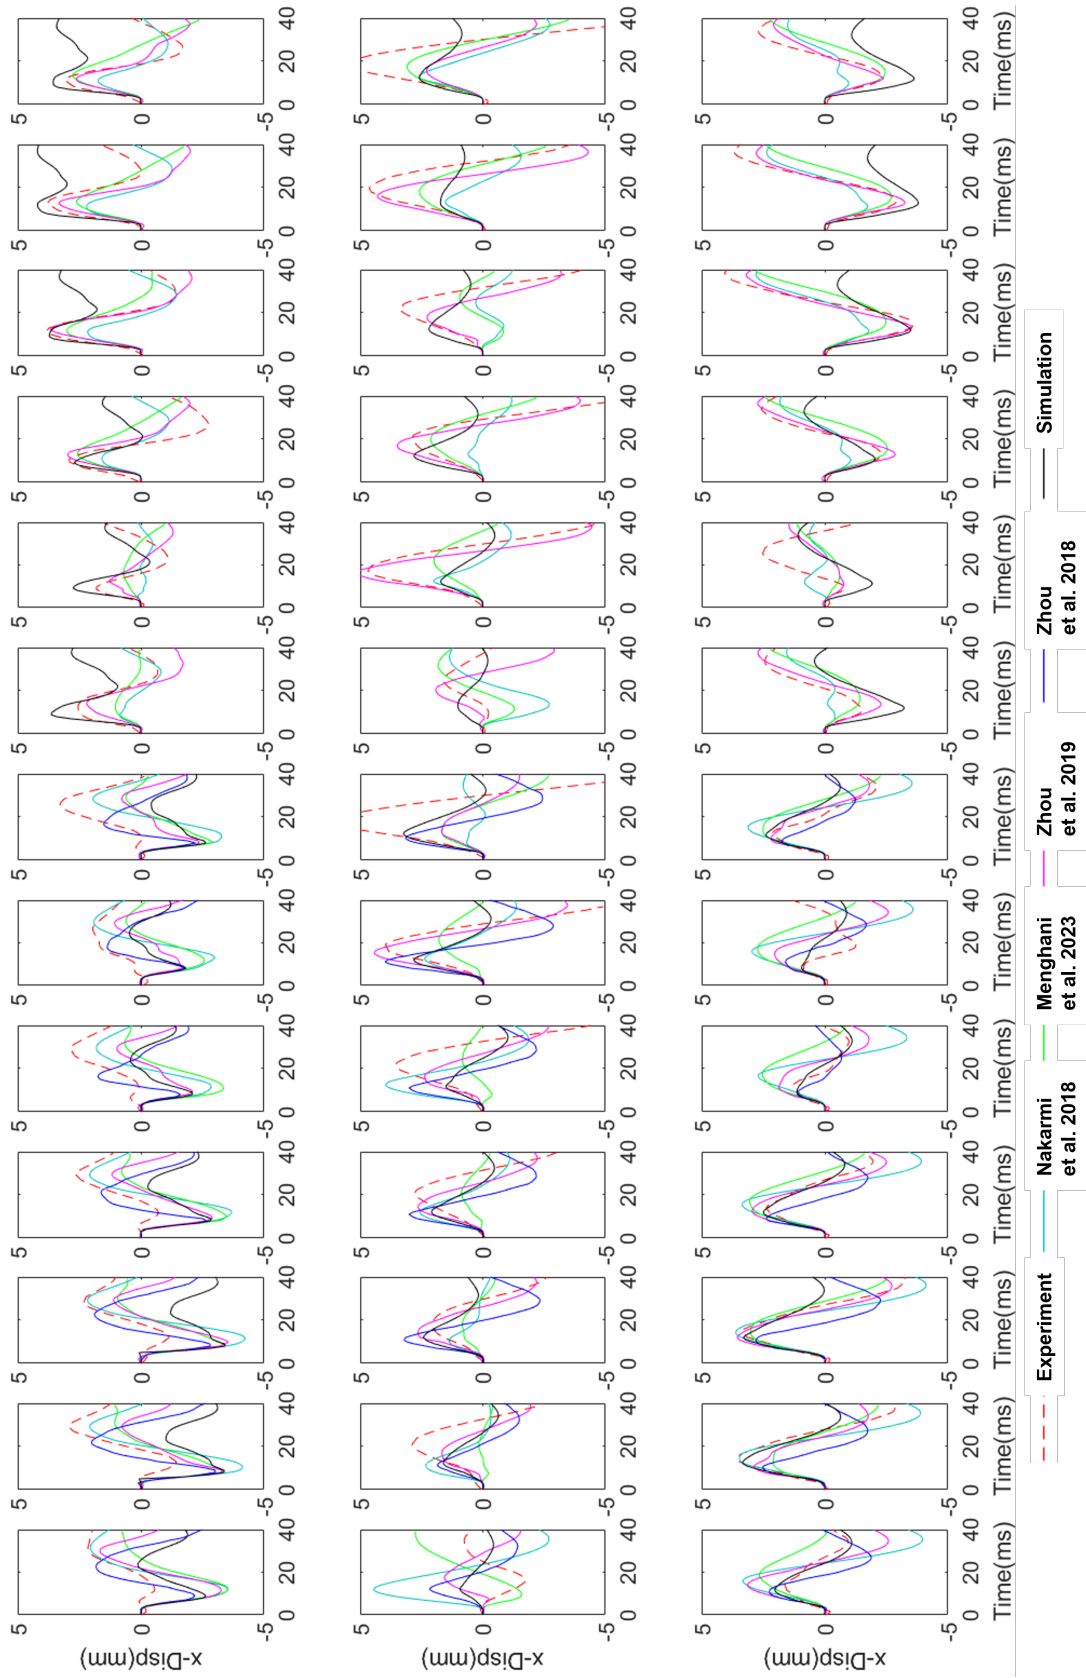

Figure S6: Comparison of NDT displacements between our simulated results and experimental results from Hardy [4] and other FEA studies [4, 6, 3, 7] for test case C380-T6.

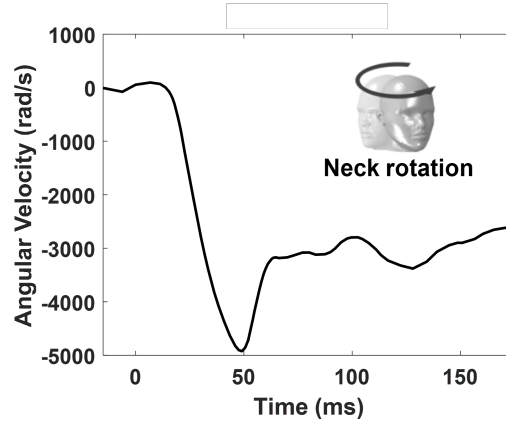

Figure S7: Angular velocity of the head for the neck rotation case.

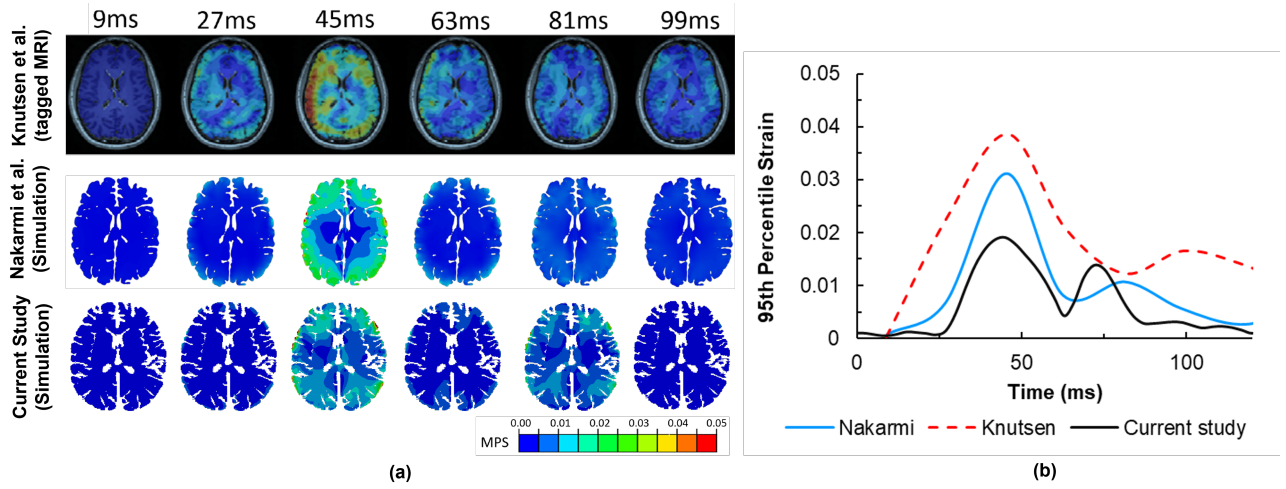

Figure S8: (a) Comparison of the evolution of MPS in the brain from the in vivo experiment [2] (top row) and our simulation (bottom two rows) ; (b) MPS95 from the experiment [2] (black) and our simulation (red).

### S2.3 Effect of CSF layer thickness on brain tissues

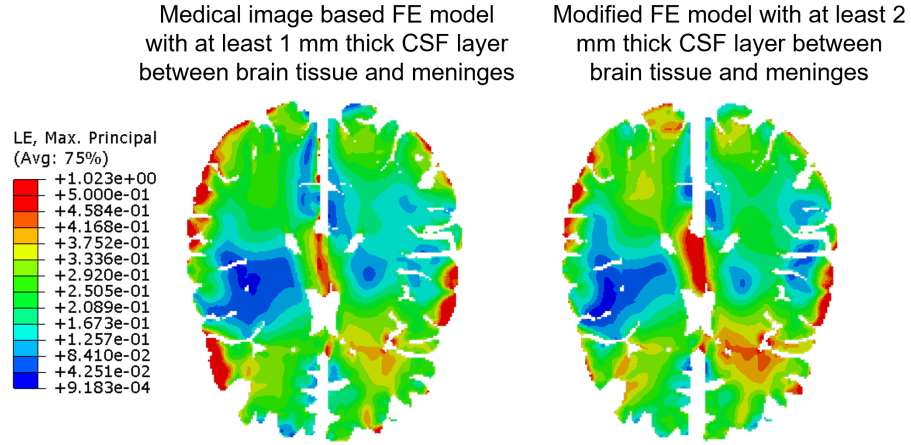

Figure S9: Maximum principal strain distribution showing the effect of CSF layer thickness. The model with thicker CSF shows higher strains near deeper brain regions and lower on the cortical surface as compared to the model with a thinner CSF layer.

## References

- [1] W. N. Hardy, M. J. Mason, C. D. Foster, C. S. Shah, J. M. Kopacz, K. H. Yang, A. I. King, J. Bishop, M. Bey, W. Anderst, et al., A study of the response of the human cadaver head to impact, *Stapp Car Crash Journal* 51 (2007) 17.
- [2] A. K. Knutsen, A. D. Gomez, M. Gangolli, W.-T. Wang, D. Chan, Y.-C. Lu, E. Christoforou, J. L. Prince, P. V. Bayly, J. A. Butman, et al., In vivo estimates of axonal stretch and 3D brain deformation during mild head impact, *Brain Multiphysics* 1 (2020) 100015.
- [3] Z. Zhou, X. Li, S. Kleiven, C. S. Shah, W. N. Hardy, A reanalysis of experimental brain strain data: implication for finite element head model validation, in: *SAE 62nd Stapp Car Crash Conference, STAPP 2018; Catamaran Resort Hotel San Diego; United States; 12 November 2018 through 14 November 2018, Vol. 2019*, SAE International, 2019.
- [4] Z. Zhou, X. Li, S. Kleiven, W. N. Hardy, Brain strain from motion of sparse markers, Tech. rep., *SAE Technical Paper* (2020).
- [5] C. Giordano, S. Kleiven, Development of an unbiased validation protocol to assess the biofidelity of finite element head models used in prediction of traumatic brain injury, Tech. rep., *SAE Technical Paper* (2016).
- [6] R. R. Menghani, A. Das, R. H. Kraft, A sensor-enabled cloud-based computing platform for computational brain biomechanics, *Computer Methods and Programs in Biomedicine* 233 (2023) 107470.
- [7] S. Nakarmi, J. Kim, L. Bezek, J. Leiding, K.-S. Lee, N. Daphalapurkar, The role of unit cell topology in modulating the compaction response of additively manufactured cellular materials using simulations and validation experiments, *Modelling and Simulation in Materials Science and Engineering* (2024).
